# Supplementary material for: Rate dependency of capillary heterogeneity trapping for CO2 storage
Source: arXiv:2511.04876 source file (2025-11-06)
Supplement: Supplementary file 1 [file SI_ArXiv.pdf]

# Supporting information for 'Rate dependency of capillary heterogeneity trapping for $CO_2$ storage'

November 6, 2025

Catrin Harris[1], Samuel Krevor[1], Ann H. Muggeridge[1], Samuel J. Jackson[2*]
[1] Department of Earth Science and Engineering, Imperial College London, London, UK.
[2] CSIRO Energy, Clayton South, Victoria, Australia.

## Abstract

This document serves as detailed supporting information for the main paper, providing extra analysis and figures to support the main findings. The section ordering is the same as the main paper. We note that figures, equations, tables and associated references from the supporting information contain the prefix S. All references without the S prefix refer to the main document.

# 1 Analytical Model Details

## 1.1 Model Derivation

The analytical model makes the following assumptions:

1. Incompressible, immiscible fluids.
2. The multiphase extension to Darcy's law applies.
3. The system is at steady state.
4. Constant rate, continuous vertically upwards flow of the wetting phase (imbibition).
5. The non-wetting phase is immobile.
6. Each layer is homogeneous (with constant $\phi$, $K$, $P_e$ defined for each layer).
7. The $k_r(S)$ and $P_c(S)$ functions have the same functional form throughout domain.
8. No wetting-phase relative permeability hysteresis (or capillary pressure hysteresis unless otherwise stated).

The derivation starts from the steady state mass conservation equation for incompressible fluids in 1-dimension,

$$\frac{\partial q_T}{\partial x} = 0, \tag{S.1}$$

*Corresponding author: Samuel J. Jackson, samuel.jackson@csiro.au

where the total flow rate $q_T$ is assumed to be a positive constant in space and time, and $x$ references a distance along the coordinate in the vertical direction (Figure 1). The system is at steady state, and hence no changes with time are considered.

Using the multiphase Darcy's law, including gravity, the wetting phase and non-wetting phase velocities are given by,

$$q_w = \frac{-Kk_{rw}}{\mu_w}(\frac{dP_w}{dx} - \rho_w g), \tag{S.2}$$

$$q_{CO2} = \frac{-Kk_{rCO2}}{\mu_{CO2}}(\frac{dP_{CO2}}{dx} - \rho_{CO2} g), \tag{S.3}$$

where $K$ is the absolute permeability, $k_r$ is the relative permeability, $\mu$ is the viscosity, $P$ is the phase pressure, $\rho$ is the density, $g$ is the component of gravitational acceleration in the vertical direction ($x$ - direction).

We define capillary pressure as,

$$P_c(S_w) = P_{CO2} - P_w, \tag{S.4}$$

The mobilities of the wetting and non-wetting phase are defined as

$$\lambda_w = \frac{k_{rw}}{\mu_w} = \frac{k_{rw}(S_{\mathrm{w}})}{\mu_w}, \tag{S.5}$$

$$\lambda_{CO2} = \frac{k_{rCO2}}{\mu_{CO2}} = \frac{k_{rCO2}(S_{\mathrm{w}})}{\mu_{CO2}}, \tag{S.6}$$

$$\lambda_T = \lambda_{CO2} + \lambda_w. \tag{S.7}$$

The porous medium is assumed to be fully saturated,

$$S_w + S_{CO2} = 1, \tag{S.8}$$

where $S_w$ and $S_{CO2}$ refer to the brine and $CO_2$ saturation respectively. In the following construction, $S$ references the wetting phase saturation unless otherwise stated. The wetting phase saturation is normalised with respect to the irreducible wetting phase saturation, $S_{wirr}$,

$$S_w^* = \frac{S_w - S_{wirr}}{1 - S_{wirr}}. \tag{S.9}$$

The connate gas saturation is assumed to be 0 throughout. Simple algebraic manipulation of the above equations results in an expression for the fractional flow of $CO_2$,

$$f_{CO2} = \frac{q_{CO2}}{q_T} = \frac{\lambda_{CO2}}{\lambda_T}(1 + \frac{\lambda_w K}{q_T}(\Delta\rho g - \frac{dP_c}{dx})). \tag{S.10}$$

As we are considering imbibition of water and the non-wetting phase is immobile, $f_{CO2} = 0$, giving

$$0 = 1 + \frac{\lambda_w K}{q_T}(\Delta\rho g - \frac{dP_c}{dx}). \tag{S.11}$$

Through substitution of the chain rule,

$$\frac{dP_c}{dx} = \frac{dP_c}{dS_w}\frac{dS_w}{dx}, \tag{S.12}$$

an expression for the saturation gradient may be obtained, where $q_T$ refers to the total wetting phase flow rate and $P_c'$ is the gradient in capillary pressure with respect to wetting-phase saturation,

$$\frac{dS_w}{dx} = \frac{\frac{q_T}{\lambda_w K} + \Delta\rho g}{P_c'}. \tag{S.13}$$

Integrating Equation S.13 over appropriate limits, we obtain the inverse solution for water saturation as a function of distance up the core is obtained,

$$\int_x^h dx = \int_{S_w}^{S_{w,critical}} \frac{P_c'}{\frac{q_T}{\lambda_w K} + \Delta\rho g} ds_w \tag{S.14}$$

## 1.2 Hysteresis

Relative permeability and capillary pressure hysteresis are important when considering imbibition processes starting from an intermediary saturation state. Non-wetting phase relative permeability hysteresis is included, necessary to capture pore-scale residual trapping processes. The analytical model (Equation 11) demonstrates $CO_2$ relative permeability has no direct impact on capillary heterogeneity trapping, other than through the pore-scale residual saturation. The capillary heterogeneity trapped saturation depends on the relative permeability of the wetting-phase. However, it has been shown experimentally to have minimal hysteresis compared with the non-wetting phase, therefore no wetting-phase relative permeability hysteresis has been included [1], [2].

The analytical solution challenges previous literature assumptions that gas relative permeability hysteresis will have dominant effects [3], demonstrating instead the leading order impact of capillary pressure hysteresis. Equation 7 shows that the form of the imbibition capillary pressure curve and the magnitude of the imbibition threshold pressure impact the capillary heterogeneity trapped saturation. Due to experimental limitations, the imbibition capillary pressure - saturation relationship is often unknown [4], [5]. Two functional forms for the imbibition capillary pressure - saturation relationship from literature were evaluated (Figure S.1a),

$$P_c^{st} = P_s \left( \frac{S_w - S_{wirr}}{1 - S_{wirr} - S_{CO2,res}^{max}} \right)^{-\frac{1}{\lambda_s}}, \tag{S.15}$$

$$P_c^{mob} = P_{ci}((1 - S_{CO2,con}^{*})^{-\frac{1}{\lambda}} - 1) + P_s. \tag{S.16}$$

The variable $P_c^{st}$ is the imbibition capillary pressure standardised to the maximum residual $CO_2$ saturation, $S_{CO2,res}^{max}$ [6], [7], where $P_s$ is the imbibition threshold pressure and $\lambda_s$ is the updated

Brooks-Corey parameter calculated based on system parameters to produce drainage and imbibition bounding curves which meet at $S_{wirr}$. The variable $P_c^{mob}$ is the imbibition capillary pressure calculated from the mobile, connected $CO_2$ saturation $S^*_{CO2,con}$ determined from residual trapping relationships [6]. $P_{ci}$ can be found through equating the drainage and imbibition capillary pressures at the turning point saturation, as outlined in Pini and Benson (2017) [8]. The imbibition threshold pressure $P_s$ is often unknown for the system of interest. In this example, $P_s$ is assumes to be a constant fraction of the drainage capillary entry pressure ($P_s = P_e/3$) [6], [9].

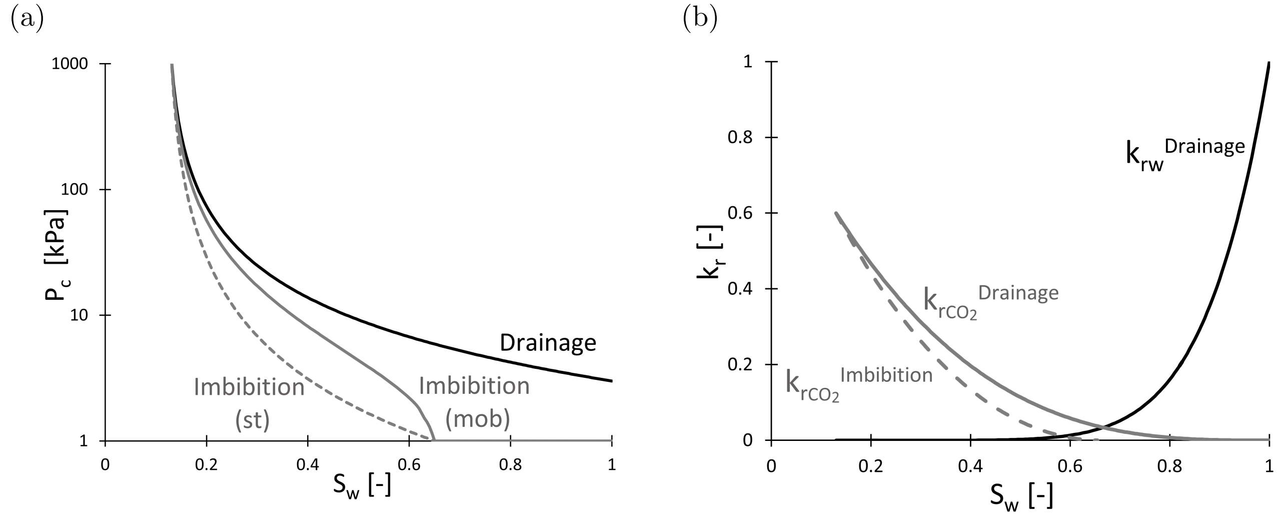


Figure S.1: (a) Capillary pressure - saturation relationships, the Brooks-Corey model for drainage alongside two potential functional forms for the imbibition capillary pressure (Equation S.15–S.16) where $P_s = P_e/3$. (b) Corey relative permeability curves, demonstrating the $CO_2$ imbibition relative permeability curve accounting only for mobile $CO_2$ saturation.

To model capillary pressure hysteresis, drainage and imbibition intrinsic capillary pressure functions are explicitly defined. The intermediate capillary pressure curves are calculated using the Killough interpolation method. Equation S.17 is used to describe hysteresis in capillary pressure when going from drainage $P_{\mathrm{c}}(D)$ to imbibition $P_{\mathrm{c}}(I)$ processes. As per Equation S.18, intermediate capillary pressure curves depend on the initial saturation at the start of the imbibition process $S_{\mathrm{TP}}$ (turning point), associated residual saturation $S_{\mathrm{res}}$ and curvature parameter $\epsilon$ typically 0.1 [10].

$$P_c(H) = \beta P_c(I) + (1 - \beta) P_c(D) \tag{S.17}$$

$$\beta = \frac{1 + \frac{\epsilon}{S_{CO2,TP} - S_{CO2,res}}}{1 + \frac{\epsilon}{Sw - (1 - S_{CO2,TP})}} \tag{S.18}$$

To model hysteresis analytically, the functional form of the intermediate capillary pressure curves calculated from Equation S.17 are substituted into Equation 11. As the hysteresis curve will vary with the turning point saturation distribution, the integration needs to be solved iteratively along the length of the system. Capillary pressure hysteresis is not included unless otherwise stated. Equation S.17 refers to capillary pressure hysteresis, however through the same process wetting-phase relative permeability hysteresis may also be accounted for.

### 1.3 Numerical simulations

The analytical model is used to validate 1D numerical simulations run using CMG IMEX, a commercial software which calculates numerical solutions to governing differential flow equations. CMG IMEX is a fully implicit, finite volume & finite difference, isothermal immiscible multiphase flow simulator [11], [12]. Small-scale models (5-6 m) on simple systems were run to demonstrate the applicability of the analytical model and the impact of dimensionless numbers. The inlet boundary condition was defined by an injection well with a constant flow rate at the bottom of the domain, and a production well at the top enforcing a constant pressure outlet boundary condition. Fluid was produced from the top at the same rate as injected, to ensure voidage replacement. Imbibition is started from a system initially at the irreducible water saturation, excluding the impact of drainage from the analysis. Brine is injected for 5 pore volumes until steady state is reached to simulate imbibition.

To demonstrate capillary heterogeneity trapping, a simple 1D heterogeneous system is defined with an upstream region of high porosity and downstream region of low porosity, representing flow upwards from a coarse to fine medium. The downstream region has a higher capillary entry pressure, as shown in Figure 1. The 1D system with regions of alternating capillary pressure, representing an idealised layered reservoir system, is used to study the impact of dimensionless trapping length on capillary heterogeneity trapping. Each grid block has its own intrinsic capillary pressure function consistent with the porosity and permeability in the heterogeneous domain, scaled according to the Leverett-J function [3], [13],

$$J(S) = \frac{P_c}{\gamma cos(\theta)}\sqrt{\frac{K}{\phi}}, \tag{S.19}$$

with interfacial tension $\gamma = 33$mN/m and contact angle $\theta = 50°$, typical values from experiment for $CO_2$-brine systems [11], [14].

Figure S.2 illustrates equivalent results are obtained through numerical simulation and analytical model over a range of brine imbibition rates. This demonstrates the validity of numerical simulator CMG IMEX to capture the physics of a heterogeneous system when capillary, gravity and viscous forces are accounted for. Figure S.2 exemplifies the inverse relationship between capillary heterogeneity trapped saturation and brine imbibition rate. The 2 region model is presented as a firm physical basis which may be extrapolated to more complex models.

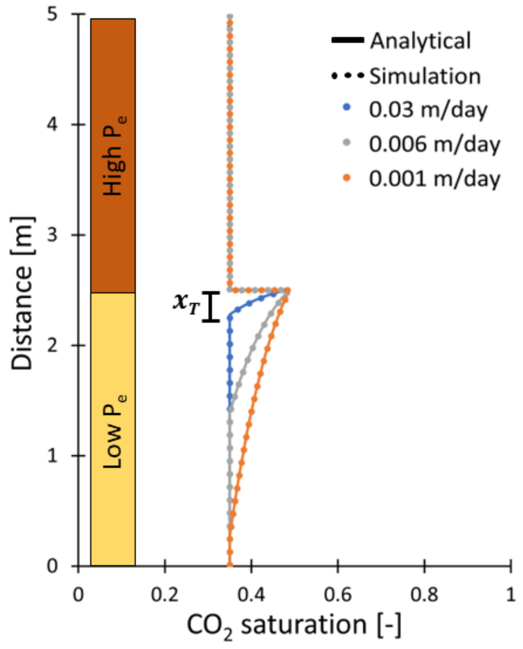


Figure S.2: An agreement between the analytical model and numerical simulation is demonstrated in a two-layer system at various imbibition rates. The final saturation post-imbibition is shown, modelled from a constant initial $CO_2$ saturation for ease of comparison. The trapping length associated with the highest flow rate is labelled.

# 2 Experimental Details

## 2.1 Experimental Workflow

1. The core is placed in a viton sleeve inside an aluminium core-holder (Bentheimer). The core-holder is secured horizontally to the medical CT scanner bed.
2. A confining pressure of 4 MPa (Bentheimer) is applied with DI water around the viton sleeve.
3. Nitrogen is injected into the core, increasing working pore-pressure to 10 MPa (Bentheimer). DI water is used to increase confining pressure to maintain a 4 MPa (Bentheimer) net overburden pressure throughout each stage of the experiment.
4. A background nitrogen scan is taken ($CT_{N2}$). Five repeat scans are taken at each stage, averaged to reduce system noise.
5. The core is depressurised and flushed with $CO_2$ (approximately 0.5 MPa) to displace in-situ nitrogen.
6. The core is flushed with DI water to displace and dissolve in-situ $CO_2$.
7. Once $CO_2$ and $N_2$ have been cleared from the system, DI water is injected into the core, increasing working pressure to set values. The confining pressure is increased accordingly.
8. DI water is flowed through the core at flow rates 2, 5 and 10 $cm^3 min^{-1}$ for the Bentheimer sample. The absolute permeability to water is measured, calculated using Darcy's law based

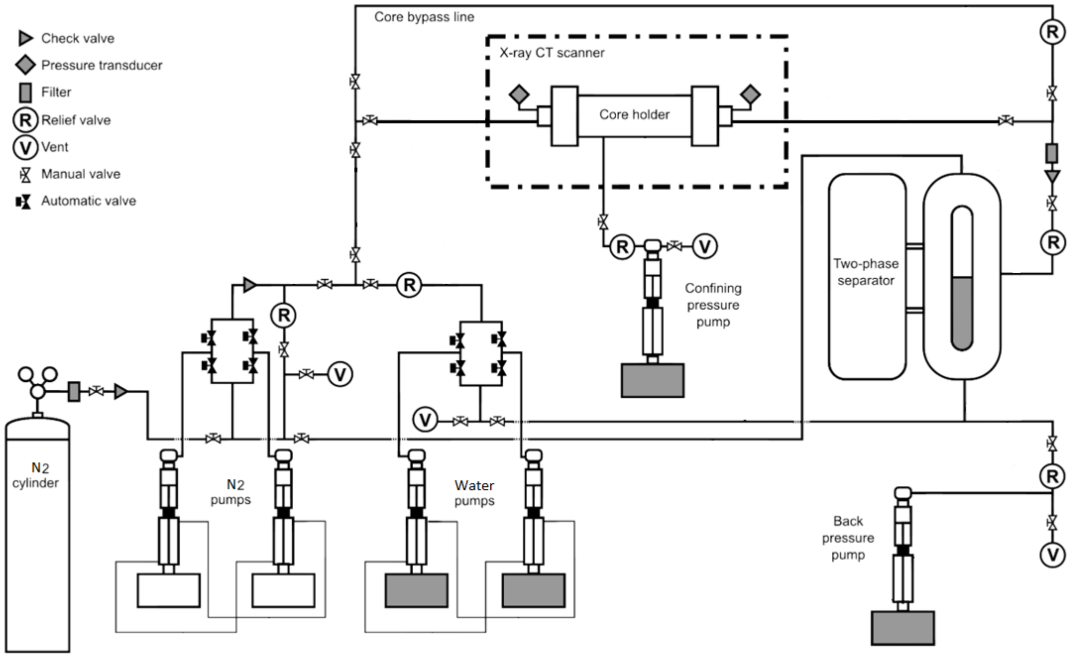


Figure S.3: Experimental flow loop used for steady-state initial-residual trapping experiments. Adapted from Reynolds et al. (2015) [15].

on the differential pressure measured across the core [6]. Absolute permeabilities are obtained across several water flow rates ($q$) to correct for the absolute pressure transducer offset. The water scans are taken (CT$_w$).

9. With system pressure maintained, drainage is performed. The sample is injected with 100% nitrogen at the flow rate detailed in Table 1 until steady state is reached (approximately 8 pore volumes). Nitrogen drainage (CT$_D$) scans are taken to record the initial saturation. During the time taken to scan the core approximately 2 additional pore volumes of nitrogen are injected, thus approximately 10 pore volumes have been injected at the imbibition start point.

10. DI water is injected into the system for approximately 1 pore volume at the designated flow rate, as specified in Table 1. Water imbibition (CT$_I$) scans are taken to record the residual saturation. Once further pore volumes of DI water are injected, dissolution starts to occur, visible in later scans.

11. Steps 5–10 are repeated to measure all flow rates in Table 1.

Further details of the experimental setup and methodology are described in [11], [15], [16]. To measure the initial-residual saturation relationship, supercritical gas and liquid phases were injected axially through the core, with the core confined in the radial direction to prevent bypass. The core is aligned horizontally along the scanner bed, due to scanner setup constraints. Gravity is expected to have negligible impact (Bond number << 1) on capillary heterogeneity trapping during the experiment. Each scan is repeated five times in immediate succession, and the average calculated to reduce error. The saturation is calculated from the CT number $S_{N_2} = (CT_{exp}–CT_w)/(CT_{N_2}–CT_w)$,

averaged over the 5 repeat scans [17]. The core is not moved between experiment and reference scans, to ensure changes in CT number are due to changes in fluid saturation.

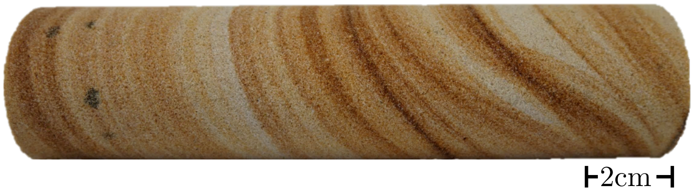


Figure S.4: Bentheimer sample (39 mm diameter, 15 cm length) with layered heterogeneities angled perpendicular to core length.

Capillary heterogeneity trapping depends on several factors: the extent of the layers, determining whether $N_2$ can bypass the layer; the contrast between the layers, determining how much $N_2$ buildup is required to satisfy capillary pressure continuity; and the relative ordering of the layers, determining how far the accumulated $N_2$ extends into the domain. Bentheimer contains layers of hematite (iron oxide deposit) visible as a distinct red colour, appearing as bright, highly attenuating patches in the CT images [18]. These iron-oxide deposits typically form around fault planes from iron-rich groundwater flow and can form between quartz grains [19]. Huang et al. (1995) find iron bands which appear as thin lamination's have an important impact on flow behaviour [20], with small throats within the banded region controlling the resistance to flow [18]. The Bentheimer sample contains a distinct layer which bisected the entire diameter of the core, with the length-scale of the heterogeneity in the direction perpendicular to flow equivalent to the core diameter. Similarly to the 1D models, this resulted in a distinct capillary barrier which needed to be overcome for fluid to move through the core.

## 2.2 Scan Error Analysis

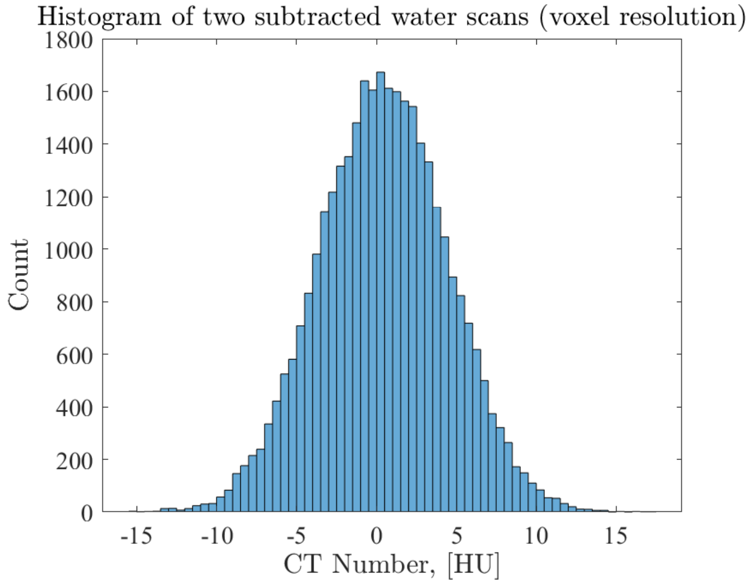


Figure S.5: Resulting distribution of subtracting two independent water scans at coarsened voxel resolution, for the Bentheimer sample.

This section outlines the X-ray CT scanner precision analysis for the current study, using the methods reported in Pini et al. (2012). For detailed equations and explanation refer to Pini et al (2012) [21]. The same medical X-ray CT scanner was used for both experiments, the Toshiba Aquilon 64 slice CT scan system at Imperial College London. Figure S.5 shows the resulting normal distribution calculated by subtracting two independent water scans at coarsened voxel resolution.

Table S.1 outlines uncertainties associated with the CT number ($\sigma_{pix}$) and calculated saturation ($\sigma_S$) for both native and coarsened voxel values, as well as slice and core averaged values obtained. Values are reported for images that are constructed from an average over 5 scans ($n = 5$), as used in the study. CT numbers assigned to each voxel are affected by an error due to the relatively small density contrast between the two fluid phases in the sample, which due to its random nature, can be reduced by combination of sufficient repeated measurements [21].

Voxel coarsening values were chosen to give the coarsened voxels well-defined Darcy-scale flow properties, with representative elementary volume (REV) similar to literature, whilst also maintaining a representative number of voxels. For a Bentheimer sandstone with similar heterogeneity, Jackson et al. (2020) find a REV of  2 mm$^3$ is suitable for porosity [6], but can be larger for multiphase properties such as saturation [22]. Pini and Madonna (2013) outline a generally accepted REV of 0.5 x 0.5 x 1 mm, which the coarsened voxels in this study were defined above [23]. The voxel-scale $N_2$ saturation values reported in this study are the coarsened voxels. The resulting voxel volumes and slice volumes are 4 mm$^3$ and 1195 mm$^3$ respectively.

| Scale | $\sigma_{pix}$ [HU] | $\sigma_s$ ([% abs.]) | |
|---|---|---|---|
| | | min | max |
| Native voxel | 6.6 | 4.5 | 6.4 |
| Coarsened voxel | 2.8 | 1.9 | 2.8 |
| Slice | - | 0.10 | 0.14 |
| Core | - | 0.008 | 0.012 |

Table S.1: Uncertainties associated with the CT number ($\sigma_{pix}$) and to the calculated saturation ($\sigma_S$) for the Bentheimer sample used in this study. The bounds account for variations in saturation throughout the experiments, with minimum saturation uncertainty corresponding to a water saturated scan and the maximum saturation uncertainty corresponding to a $N_2$ saturated scan.

Comparing Table S.1 to the results in Pini et al. (2012), the uncertainties are a similar order of magnitude [21]. Pini et al. (2012) found the random error was 4.9–5.9% for 6.25 mm$^3$ voxels, which reduced to $< 0.3\%$ for slice average saturations. Similarly, Ni (2019) found over a wide range of sandstones the random error was 7.9–9.8% for 10 mm$^3$ voxels, which reduced to 0.22–0.3% for slice average saturations, using a differential imaging medical CT setup. The uncertainty in the voxel-level saturation is already significantly reduced through coarsening. Slice-averaged values all have very low uncertainty with even less uncertainty in the core-averaged data, meaning at core level, any uncertainty due to CT scanner measurement precision can be ignored [24].

## 2.3 Saturation Distribution

The experimental slice average $N_2$ saturation along the core length is shown in Figure S.6. The initial saturation at the start of the imbibition process is represented by the solid lines. As drainage was repeated under the same conditions, we should expect to see similar initial saturations between the

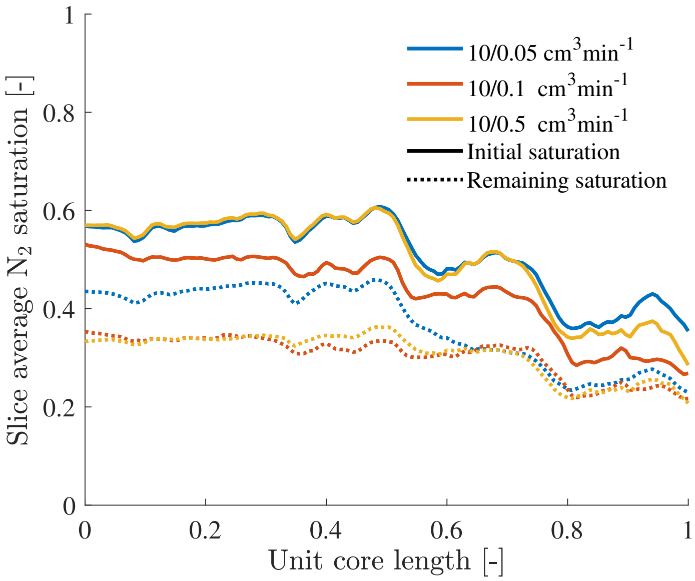


Figure S.6: Slice average saturation (initial = solid line, remaining = dotted line) along unit core length for the Bentheimer sample. Three different imbibition flow rate experiments are shown, with a constant drainage flow rate of 10 $cm^3min^{-1}$ between experiments.

experiment repeats. Indeed, a good match is observed between drainage runs 1 and 3, however a lower drainage saturation was observed on run 2, likely due to a lower number of pore volumes injected. The final saturation observed on imbibition is represented by the dotted lines. The saturation distribution is impacted during both drainage and imbibition by the layered heterogeneities within the core, in particular by the low porosity band just over half way along the core. The low porosity band is observed, Figure 2, to intersect the entire core diameter. A build-up of nitrogen is observed behind the region of low porosity, during both drainage and imbibition.

The 3D voxel average initial and residual $N_2$ saturation are shown in Figure S.7. Figure S.7 shows clearly the impact of the low porosity band, resulting in stark differences in saturation distribution around the heterogeneity for the Bentheimer sample. Note, drainage from repeat 0.1$cm^3min^{-1}$ is shifted relative to the other flow rate repeats due to experimental complications meaning full 10 PV drainage was not complete, instead estimated 8–9 PV were injected in total. This is expected to have limited impact on the results as the comparison of initial to residual saturation is key.

## 2.4 Land and Linear Trapping Coefficient

The maximum Land trapping coefficient is calculated by fitting the slice average initial-residual data for the high flow rate (0.5 $cm^3min^{-1}$) experiment, Figure S.8a. The slice average saturations are used to parameterise the Land trapping model as they are above the saturation REV, capturing intrinsic trapping. Isolating the high flow rate experimental data, a Land trapping coefficient $C = 1.24 \pm 0.13$ is found to fit the data (1 standard deviation of uncertainty).

Capillary heterogeneity trapping impacts the shape of the initial-residual trapping characteristics. The Land model is observed to describe well the data trend for the slice average initial-residual $N_2$ saturation at high flow rate. Figure S.8b shows the low flow rate (0.05 $cm^3min^{-1}$) data only. The lower bound Linear trapping curve ($A = 0.62$), average Linear trapping curve ($A = 0.71$) and

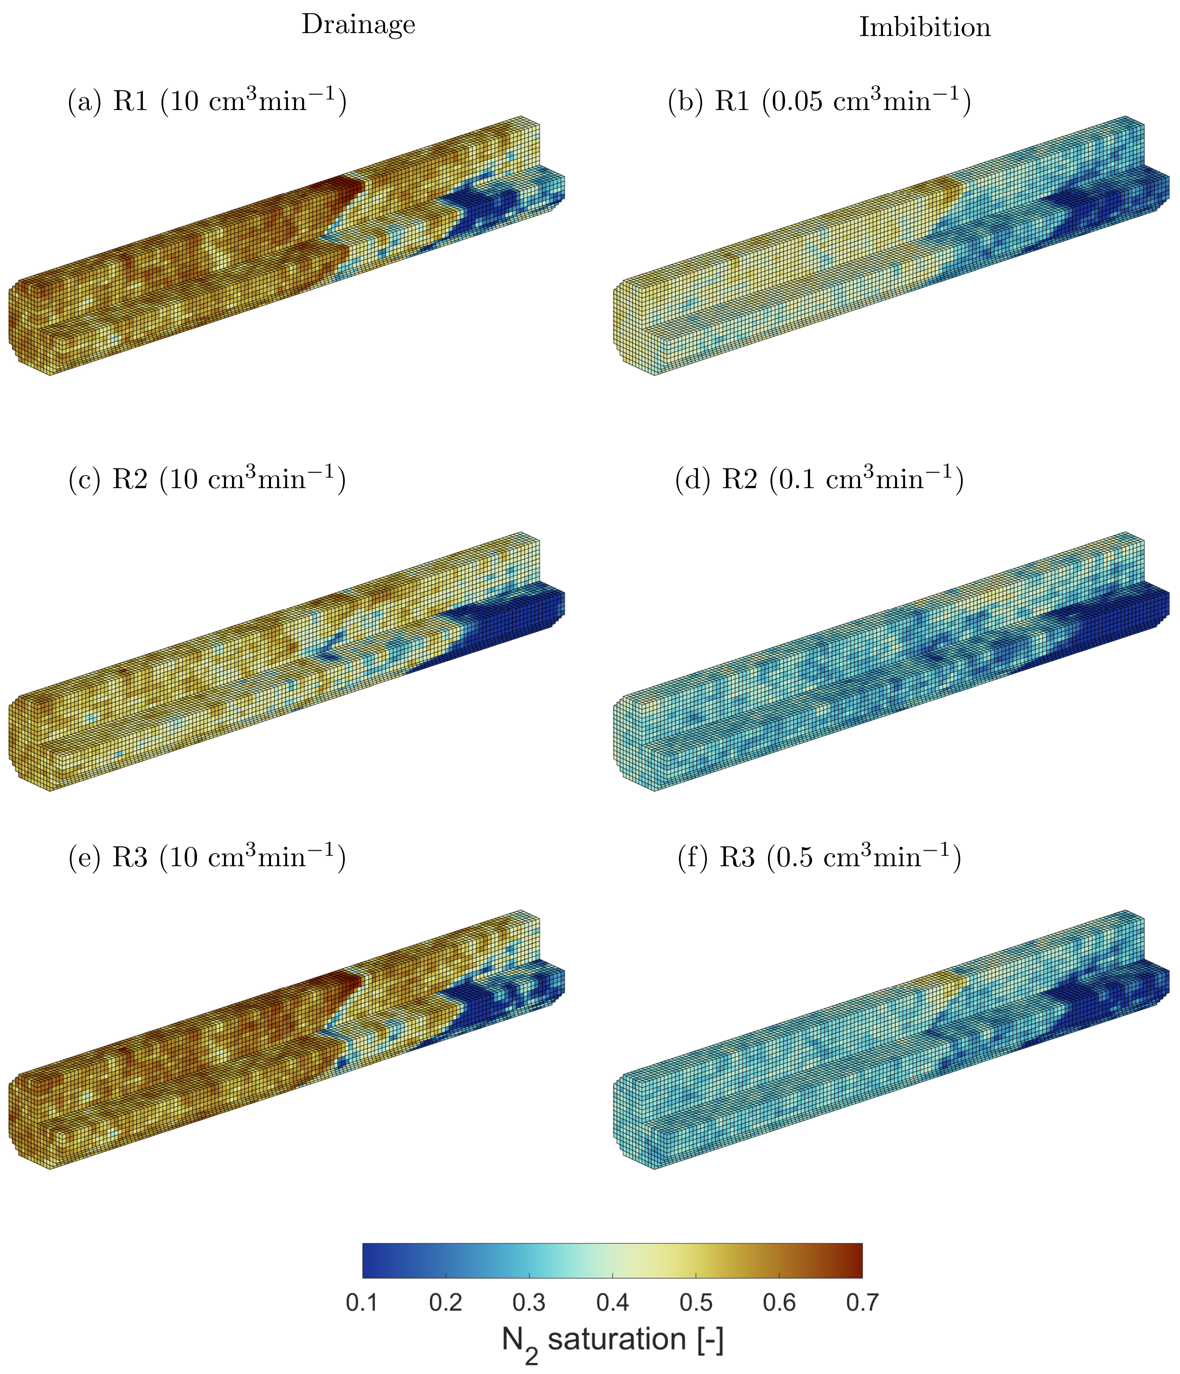


Figure S.7: Initial-residual $N_2$ saturation in the Bentheimer sample for three flow rate experiments, displayed in 3D. The $N_2$ saturation distribution's on drainage (initial saturation) are displayed on the left hand side and the $N_2$ saturation distribution's on imbibition (remaining saturation) on the right hand side.

Linear trapping curve upstream of the heterogeneity ($A = 0.76$) are displayed. The linear trapping coefficient is shown to fit well to the data at low flow rate, implying the Land correlation may not be the best parameterisation in systems dominated by capillary heterogeneity trapping.

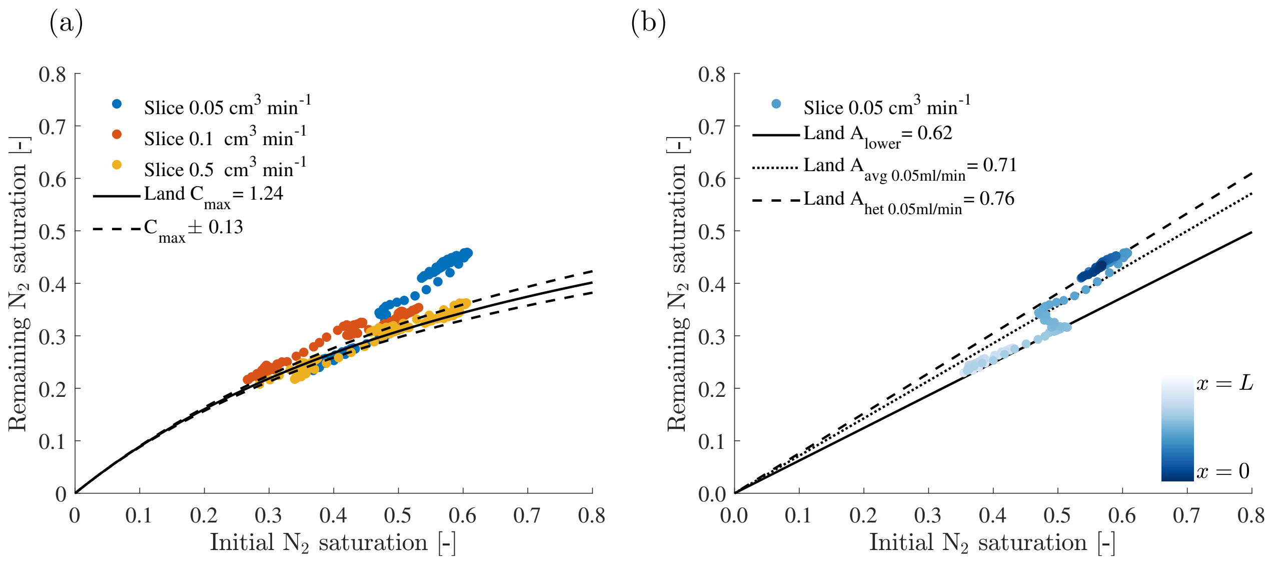


Figure S.8: (a.) Slice average initial-residual $N_2$ saturation for three flow rate experiments in the Bentheimer sample. The maximum Land trapping relationship plotted with ± 1 standard deviation of uncertainty ($C = 1.24$, $C^{-} = 1.11$, $C^{+} = 1.37$). (b.) Slice average initial-residual $N_2$ saturation for the low flow rate (0.05 cm$^3$min$^{-1}$) experiment. The lower bound Linear trapping curve (solid line), average Linear trapping curve (dotted line) and Linear trapping curve upstream of the heterogeneity (dashed line) are displayed.

### 2.4.1 Voxel-level saturation

The individual voxel saturation shows a similar trend to the slice average saturations, with a distinct relationship for each flow rate experiment observed. The voxel-scale data is more disperse, whilst averaging over the slice reduces the spread in the data. Figure S.9 shows the voxel saturations overlaid by the slice average saturations for each flow rate experiment. The colour gradient demonstrates the position of the saturation along the core length. It is observed that higher initial saturations occur at the core inlet. This is likely due to a combination of both saturation build up upstream of the main heterogeneity during drainage and the capillary end effect which results in a capillary pressure gradient decreasing towards the outlet of the core [6], [17], [25]. Variations in the saturation at the coarsened voxel size are larger than the uncertainty in saturation measurements from X-ray CT scanning ($< 3\%$), implying the scatter results from the inherent REV of the saturation (Appendix 2.2). At the slice average scale the uncertainty in saturation measurements from X-ray CT scanning is reduced further ($< 0.15\%$), confirming the observed variations in trapping at this scale are due to REV scale heterogeneities in capillary pressure, indicative of capillary heterogeneity trapping.

### 2.4.2 Literature Comparison

As a laboratory standard rock, there have previously been many experiments carried out on Bentheimer samples, often on homogeneous specimen. The experiments in Jackson et al. (2020) are carried out on cm-scale core's with decane and brine as working fluids. A total flow rate of 0.1 cm$^3$min$^{-1}$ flooded the core during both drainage and imbibition, with the pore scale capillary number 2.2x10$^{-7}$ at the end of drainage, larger than the capillary number used for any of the experiments performed here. The voxel volume, 6.8 mm$^3$, was the same order of magnitude as these experiments, however the slice volume, 171 mm$^3$, was an order of magnitude lower due to the

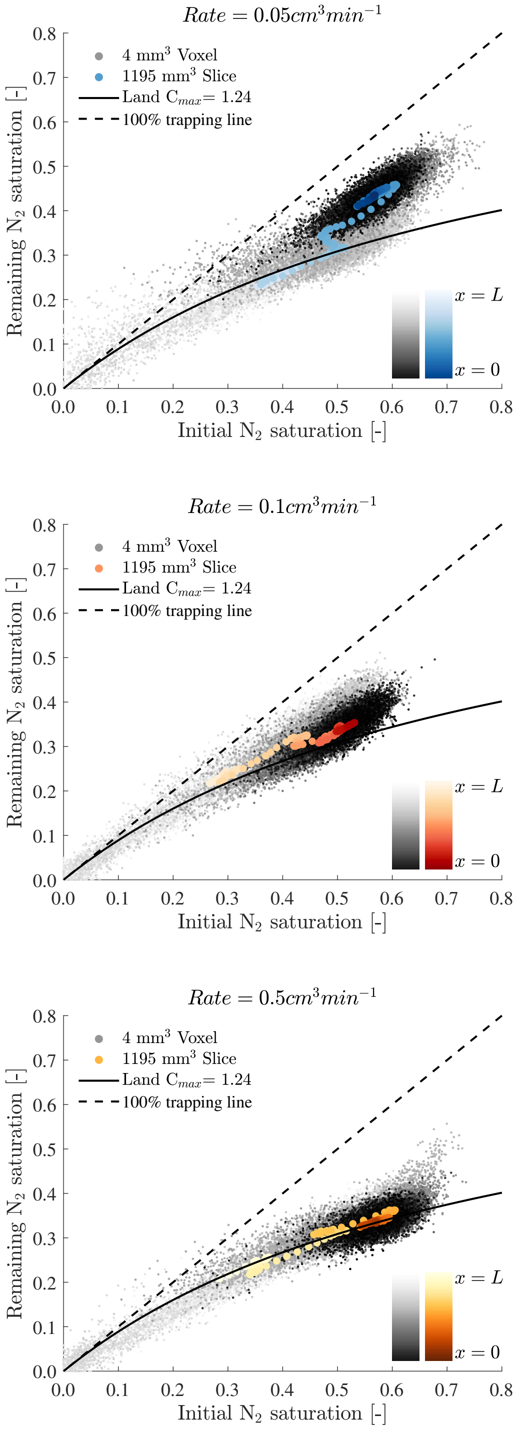


Figure S.9: Initial-residual saturation at slice average and voxel-scale for three rates (0.05 $cm^3min^{-1}$, 0.1 $cm^3min^{-1}$, 0.5 $cm^3min^{-1}$) in the Bentheimer sample. The colour gradient shows where along the core from inlet ($x$=0) to outlet ($x$=$L$) the saturations occur.

smaller core size.

The results from Jackson et al. (2020) are considered as analogous homogeneous and heterogeneous

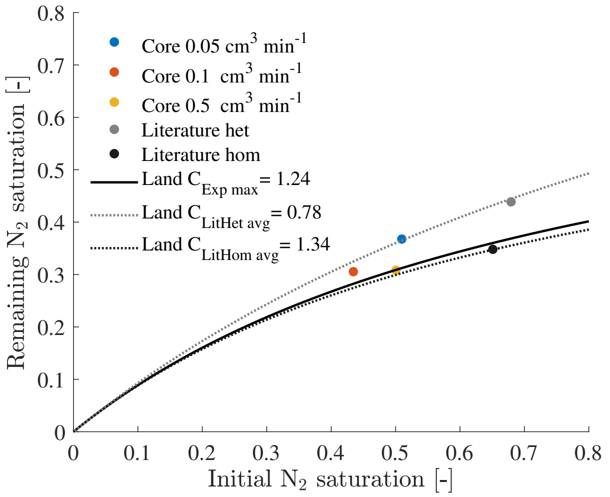


Figure S.10: Core average initial-residual $N_2$ saturation for three flow rate experiments. In addition literature comparisons from Jackson et al. (2020) for a homogeneous and heterogeneous Bentheimer [6]. The maximum experimental Land trapping coefficient $C = 1.24$ (solid line) is displayed, in addition to the average trapping relationship for the comparison homogeneous $C = 1.34$ and heterogeneous $C = 0.78$ literature samples (dotted lines).

experiments. Figure S.10 demonstrates the initial-residual trapping relationship may behave more similarly to a heterogeneous or homogeneous sample dependent on flow conditions used. At the core-scale the low flow rate experiment obeys a similar trapping relationship to the heterogeneous literature sample, whilst the high flow rate experiment obeys a similar trapping relationship to the homogeneous literature sample.

Figure S.11a demonstrates a good agreement in trapping behaviour at voxel and slice scale between the high flow rate (0.5 $\text{cm}^3\text{min}^{-1}$) experiment and Jackson et al. (2020) homogeneous experiment. The best fit maximum Land coefficient calculated from the Imperial College London experiments (slice average from high flow rate 0.5 $\text{cm}^3\text{min}^{-1}$ experiment) is $C = 1.24 \pm 0.13$ (1 standard deviation). As seen in Figure S.11a, this has a similar trapping relationship to the homogeneous experiment from Jackson et al. (2020), which has a best fit Land correlation (slice average) of $C = 1.34 \pm 0.12$ (1 standard deviation), with both curves falling within the experimental error of the other.

In Figure S.11b the slice average and voxel-scale initial-residual saturation data from the low flow rate experiment (0.05 $\text{cm}^3\text{min}^{-1}$) is isolated and compared to the heterogeneous Bentheimer sample from Jackson et al. (2020) [6]. Jackson et al. (2020) use a lower Land trapping coefficient of $C = 0.5$ to parameterise trapping in the heterogeneous Bentheimer. This trapping relationship is comparable to the low flow rate experiment (0.05 $\text{cm}^3\text{min}^{-1}$) fitted upstream of the heterogeneity $C = 0.55 \pm 0.05$. Figure S.11b demonstrates a good agreement between the trapping relationship in this region ($S_{res,N2} \sim 0.45 - 0.65$). Differences between the trapping relationships occur due to differences in the heterogeneities between the cores.

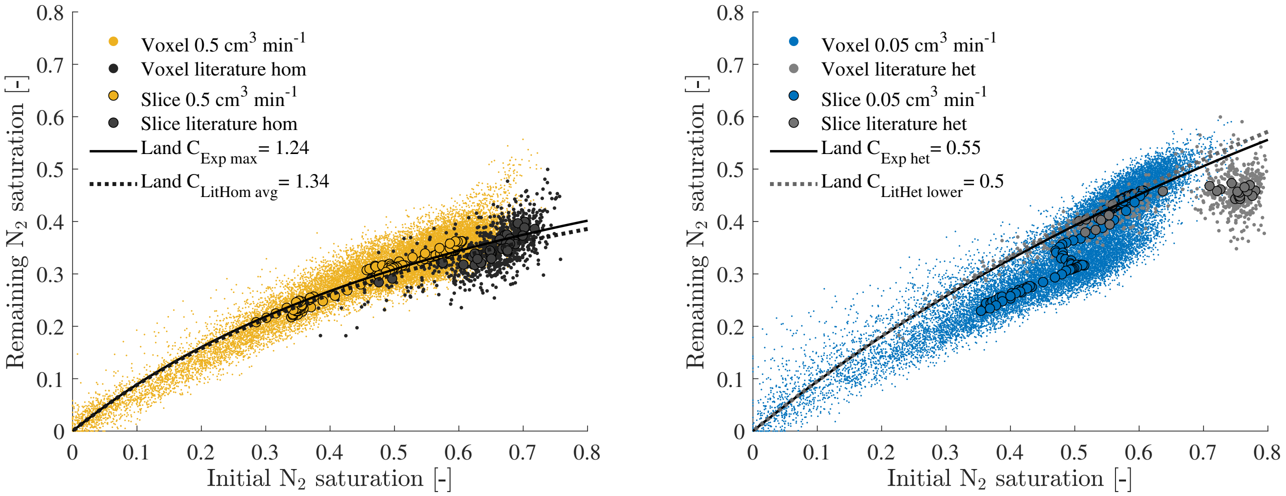


Figure S.11: (a.) Slice average and voxel-scale initial-residual $N_2$ saturation for the high flow rate (0.5 $cm^3 min^{-1}$) experiment and the homogeneous sample from Jackson et al. (2020) [6]. The average Land trapping coefficient for the high flow rate experiment (equivalent to the maximum Land trapping coefficient across the different flow rates) $C = 1.24$ (solid line) and average Land trapping coefficient for the homogeneous literature comparison $C = 1.34$ (dotted line) are displayed. (b.) Slice average and voxel-scale initial-residual $N_2$ saturation for the low flow rate (0.05 $cm^3 min^{-1}$) experiment and the heterogeneous sample from Jackson et al. (2020) [6]. The lower Land trapping coefficient for the low flow rate experiment (calculated as the average trapping relationship upstream of the heterogeneity) $C = 0.55$ (solid line) and lower Land trapping coefficient for the heterogeneous literature comparison $C = 0.5$ (dotted line) are displayed.

# References


[1] G. R. Jerauld and S. J. Salter, "The effect of pore-structure on hysteresis in relative permeability and capillary pressure: pore-level modeling," *Transport in Porous Media*, vol. 5, no. 2, pp. 103–151, 1990. DOI: 10.1007/BF00144600.

[2] R. Juanes, E. J. Spiteri, F. M. Orr, and M. J. Blunt, "Impact of relative permeability hysteresis on geological $CO_2$ storage," *Water Resources Research*, vol. 42, no. 12, W12418, 2006. DOI: 10.1029/2005WR004806.

[3] E. Saadatpoor, S. L. Bryant, and K. Sepehrnoori, "New Trapping Mechanism in Carbon Sequestration," *Transport in Porous Media*, vol. 82, no. 1, pp. 3–17, 2010. DOI: 10.1007/s11242-009-9446-6.

[4] C. Zahasky and S. M. Benson, "Spatial and Temporal Quantification of Spontaneous Imbibition," *Geophysical Research Letters*, vol. 46, no. 21, pp. 11 972–11 982, 2019. DOI: 10.1029/2019GL084532.

[5] M. J. Blunt, *Multiphase flow in permeable media: A pore-scale perspective*. Cambridge University Press, 2017.

[6] S. Jackson, Q. Lin, and S. Krevor, "Representative Elementary Volumes, Hysteresis and Heterogeneity in Multiphase Flow From the Pore to Continuum Scale," *Water Resources Research*, vol. 56, no. 6, e2019WR026396, 2020. DOI: 10.1029/2019wr026396.

[7] M. H. Sedaghat and S. Azizmohammadi, "Representative-Elementary-Volume Analysis of Two-Phase Flow in Layered Rocks," *SPE Reservoir Evaluation and Engineering*, vol. 22, no. 3, pp. 1075–1083, 2019. DOI: 10.2118/194014-PA.

[8] R. Pini and S. M. Benson, "Capillary pressure heterogeneity and hysteresis for the supercritical $CO_2$/water system in a sandstone," *Advances in Water Resources*, vol. 108, pp. 277–292, 2017. DOI: 10.1016/j.advwatres.2017.08.011.

[9] B. Raeesi, N. R. Morrow, and G. Mason, "Capillary Pressure Hysteresis Behavior of Three Sandstones Measured with a Multistep Outflow-Inflow Apparatus," *Vadose Zone Journal*, vol. 13, no. 3, pp. 1–12, 2014. DOI: 10.2136/vzj2013.06.0097.

[10] J. E. Killough, "Reservoir simulation with history-dependent saturation functions.," *Society of Petroleum Engineers Journal*, vol. 16, no. 1, pp. 37–48, 1976. DOI: 10.2118/5106-PA.

[11] S. J. Jackson and S. Krevor, "Small-Scale Capillary Heterogeneity Linked to Rapid Plume Migration During $CO_2$ Storage," *Geophysical Research Letters*, vol. 47, no. 18, e2020GL088616, 2020. DOI: 10.1029/2020GL088616.

[12] CMG IMEX, *Advanced Oil/Gas Reservoir Simulator Version 2000 User's Guide*. Calgary, Alberta: Computer Modelling Group LTD., 2000.

[13] M. C. Leverett, "Capillary Behavior in Porous Solids," *Transactions of the AIME*, vol. 142, no. 1, pp. 152–169, 1941. DOI: 10.2118/941152-G.

[14] S. Benson, R. Pini, C. Reynolds, and S. Krevor, "Relative permeability analyses to describe multi-phase flow in $CO_2$ storage reservoirs," Global CCS Institute, GCCSI Report 2, 2013. [Online]. Available: https://www.globalccsinstitute.com/archive/hub/publications/111691/relative-permeability-analysis-describe-multi-phase-flow-co2-storage-reservoirs.pdf.

[15] C. A. Reynolds and S. Krevor, "Characterizing flow behavior for gas injection: Relative permeability of $CO_2$-brine and $N_2$-water in heterogeneous rocks," *Water Resources Research*, vol. 51, no. 12, pp. 9464–9489, 2015. DOI: 10.1002/2015WR018046.

[16] S. J. Jackson, S. Agada, C. A. Reynolds, and S. Krevor, "Characterizing Drainage Multiphase Flow in Heterogeneous Sandstones," *Water Resources Research*, vol. 54, no. 4, pp. 3139–3161, 2018. DOI: 10.1029/2017WR022282.

[17] S. C. Krevor, R. Pini, L. Zuo, and S. M. Benson, "Relative permeability and trapping of $CO_2$ and water in sandstone rocks at reservoir conditions," *Water Resources Research*, vol. 48, no. 2, pp. 1–16, 2012. DOI: 10.1029/2011WR010859.

[18] S. J. Jackson, Y. Niu, S. Manoorkar, P. Mostaghimi, and R. T. Armstrong, "Deep Learning of Multiresolution X-Ray Micro-Computed-Tomography Images for Multiscale Modeling," *Physical Review Applied*, vol. 17, no. 5, p. 054 046, 2022. DOI: 10.1103/PhysRevApplied.17.054046.

[19] C. Wim Dubelaar and T. G. Nijland, "The bentheim sandstone: Geology, petrophysics, varieties and its use as dimension stone," in *Engineering Geology for Society and Territory - Volume 8*, G. Lollino, D. Giordan, C. Marunteanu, B. Christaras, I. Yoshinori, and C. Margottini, Eds., Springer, Cham, 2015. DOI: 10.1007/978-3-319-09408-3_100.

[20] Y. Huang, P. S. Ringrose, and K. S. Sorbie, "Capillary Trapping Mechanisms in Water-Wet Laminated Rocks," *SPE Reservoir Engineering*, vol. 10, no. 04, pp. 287–292, 1995. DOI: 10.2118/28942-PA.

[21] R. Pini, S. C. Krevor, and S. M. Benson, "Capillary pressure and heterogeneity for the $CO_2$/water system in sandstone rocks at reservoir conditions," *Advances in Water Resources*, vol. 38, pp. 48–59, 2012. DOI: 10.1016/j.advwatres.2011.12.007.

[22] A. L. Herring, E. J. Harper, L. Andersson, A. Sheppard, B. K. Bay, and D. Wildenschild, "Effect of fluid topology on residual nonwetting phase trapping: Implications for geologic $CO_2$ sequestration," *Advances in Water Resources*, vol. 62, pp. 47–58, 2013. DOI: 10.1016/j.advwatres.2013.09.015.

[23] R. Pini and S. M. Benson, "Simultaneous determination of capillary pressure and relative permeability curves from core-flooding experiments with various fluid pairs," *Water Resources Research*, vol. 49, no. 6, pp. 3516–3530, 2013. DOI: 10.1002/wrcr.20274.

[24] H. Ni, M. Boon, C. Garing, and S. M. Benson, "Predicting $CO_2$ residual trapping ability based on experimental petrophysical properties for different sandstone types," *International Journal of Greenhouse Gas Control*, vol. 86, pp. 158–176, 2019. DOI: 10.1016/j.ijggc.2019.04.024.

[25] B. Niu, A. Al-Menhali, and S. C. Krevor, "The impact of reservoir conditions on the residual trapping of carbon dioxide in Berea sandstone," *Water Resources Research*, vol. 51, no. 4, pp. 2009–2029, 2015. DOI: 10.1002/2014WR016441.
